# Supplementary material for: Transmissive Beyond Diagonal RIS-Mounted LEO Communication for NOMA IoT Networks
Source: arXiv:2501.02742 source file (2025-02-22)

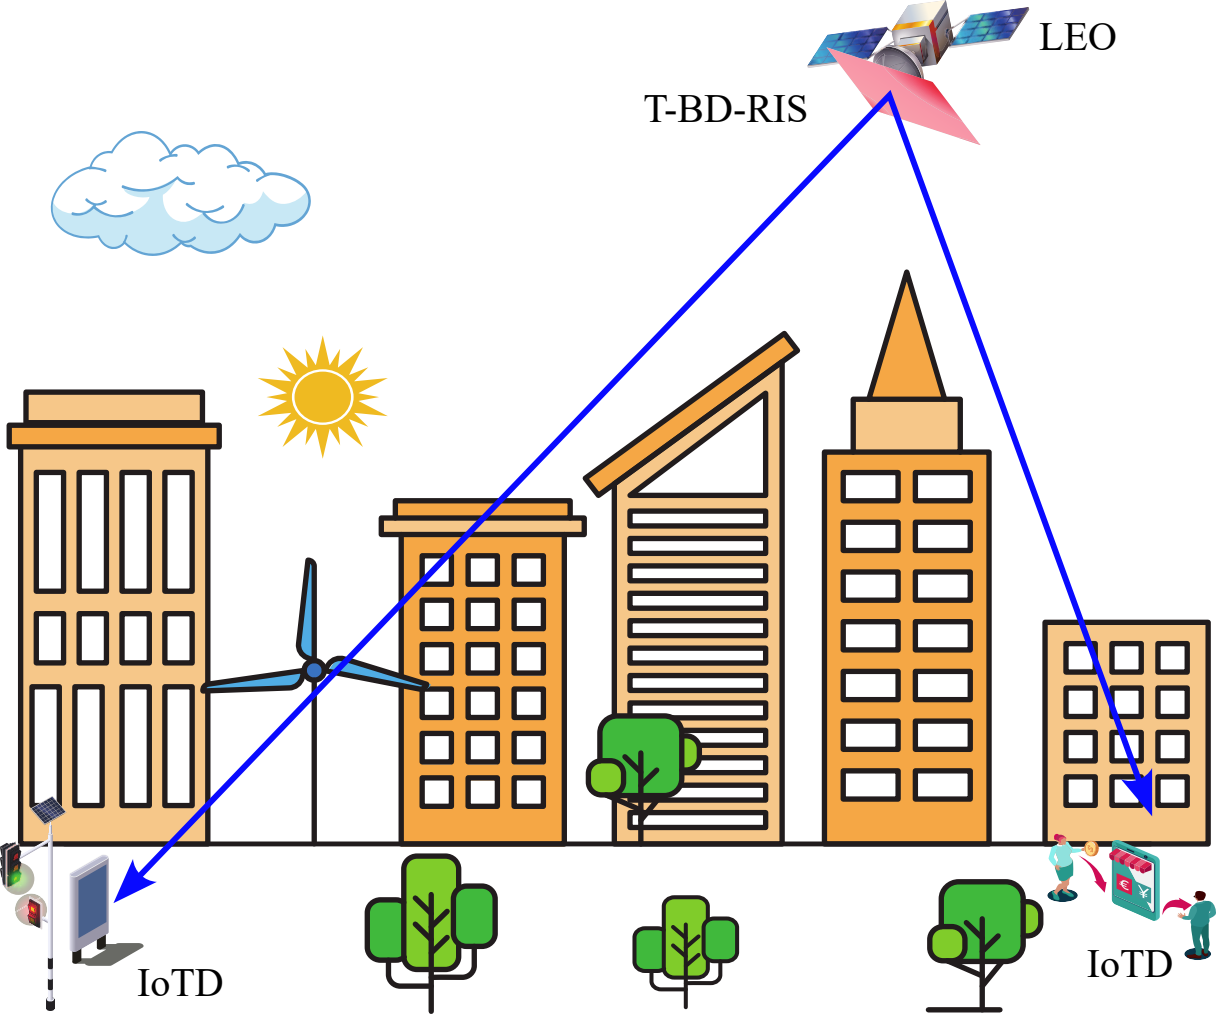

Supplement: Supplementary file 1 [file SM.pdf]
